# Supplementary material for: Electron Spin Resonance of Defects in Spin Chains. o-(DMTTF)2X : a versatile system behaving like molecular magnet
Source: arXiv:2008.10897 ancillary file (2020-08-25)
Supplement: Supplementary file 1 [file Supplementary.pdf]

# Electron Spin Resonance of Defects in Spin Chains

# o-$(DMTTF)_2X$ : a versatile system behaving like molecular magnet} Supplementary Informations

Loic Soriano · Julian Zeisner · Vladislav Kataev · Marc Fourmigue · Olivier Jeannin · Herve Vezin · Maylis Orio · Sylvain Bertaina*

## Theoretical Results DFT

### $[(DMTTF)_2I_8]^{5-}$

| $g_{min}$ | $g_{mid}$ | $g_{max}$ | $g_{iso}$ |
|---|---|---|---|
| 2.00219 | 2.01044 | 2.01182 | 2.00815 |

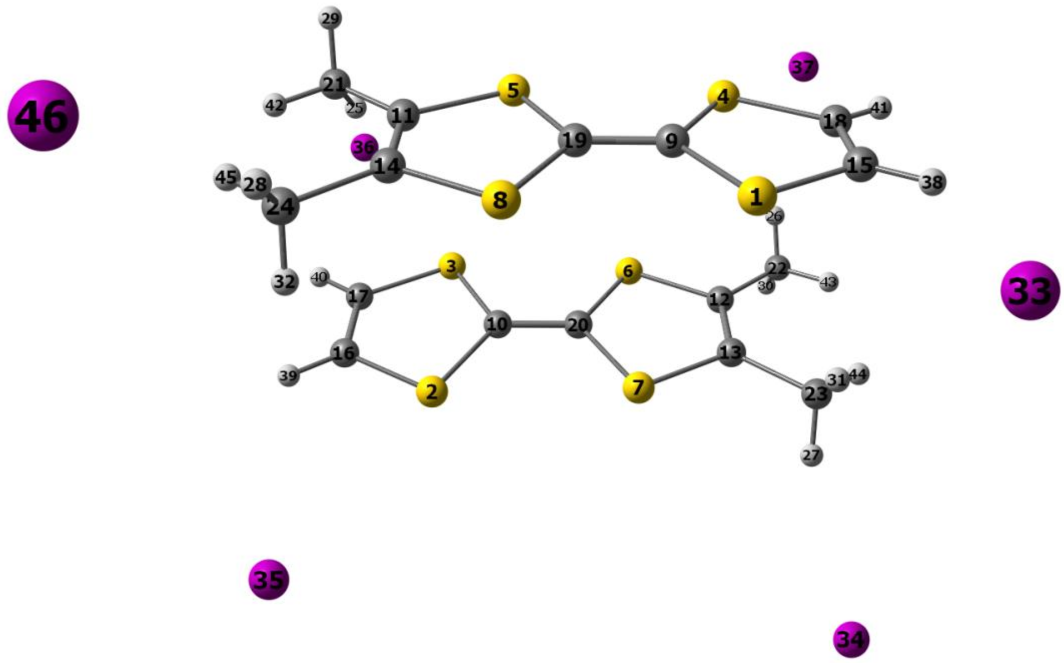


| Center | $A_{min}$ | $A_{mid}$ | $A_{max}$ | $A_{iso}$ |
|---|---|---|---|---|
| S1 | -3.7 | -4.5 | 26.6 | 6.2 |

| Center | $A_{min}$ | $A_{mid}$ | $A_{max}$ | $A_{iso}$ |
|---|---|---|---|---|
| S2 | -3.7 | -4.5 | 26.6 | 6.2 |
| S3 | -2.7 | -3.3 | 23.5 | 5.8 |
| S4 | -2.7 | -3.3 | 23.5 | 5.8 |
| S5 | -1.8 | -2.7 | 22.2 | 5.9 |
| S6 | -1.8 | -2.7 | 22.2 | 5.9 |
| S7 | -2.2 | -3.2 | 22.6 | 5.8 |
| S8 | -2.2 | -3.2 | 22.6 | 5.8 |

| Center | $A_{min}$ | $A_{mid}$ | $A_{max}$ | $A_{iso}$ |
|---|---|---|---|---|
| I33 | 4.1 | 4.9 | 6.4 | 5.1 |
| I34 | 1.9 | 1.9 | 2.6 | 2.1 |
| I35 | 4.1 | 4.9 | 6.4 | 5.1 |
| I36 | -0.4 | -0.8 | -1.0 | -0.8 |
| I37 | -0.4 | -0.8 | -1.0 | -0.8 |
| I46 | 1.9 | 1.9 | 2.6 | 2.1 |

| Center | $A_{min}$ | $A_{mid}$ | $A_{max}$ | $A_{iso}$ |
|---|---|---|---|---|
| C9 | -4.4 | -5.4 | 17.9 | 2.7 |
| C10 | -4.4 | -5.4 | 17.9 | 2.7 |
| C11 | -1.5 | -1.9 | 5.0 | 0.5 |
| C12 | -1.5 | -1.9 | 5.0 | 0.5 |
| C13 | 1.2 | -2.0 | -2.4 | -1.1 |
| C14 | 1.2 | -2.0 | -2.4 | -1.1 |
| C15 | 1.6 | -2.3 | -2.5 | -1.1 |
| C16 | 1.6 | -2.3 | -2.5 | -1.1 |

| Center | $A_{min}$ | $A_{mid}$ | $A_{max}$ | $A_{iso}$ |
|---|---|---|---|---|
| C17 | -2.2 | -2.4 | 3.3 | -0.4 |
| C18 | -2.2 | -2.4 | 3.3 | -0.4 |
| C19 | -5.1 | -6.2 | 13.2 | 0.6 |
| C20 | -5.1 | -6.2 | 13.2 | 0.6 |
| C21 | -0.6 | -0.8 | -0.9 | -0.8 |
| C22 | -0.6 | -0.8 | -0.9 | -0.8 |
| C23 | -0.3 | -0.5 | -0.7 | -0.5 |
| C24 | -0.3 | -0.5 | -0.7 | -0.5 |

| Center | $A_{min}$ | $A_{mid}$ | $A_{max}$ | $A_{iso}$ |
|---|---|---|---|---|
| H25 | 1.3 | 1.8 | 3.0 | 2.0 |
| H26 | 1.3 | 1.8 | 3.0 | 2.0 |
| H27 | 0.1 | 0.2 | 1.5 | 0.6 |
| H28 | 0.1 | 0.2 | 1.5 | 0.6 |
| H29 | 1.1 | 1.2 | 2.6 | 1.6 |
| H30 | 1.1 | 1.2 | 2.6 | 1.6 |
| H31 | 0.6 | 1.1 | 2.2 | 1.3 |
| H32 | 0.6 | 1.1 | 2.2 | 1.3 |
| H38 | 0.4 | -2.0 | -2.5 | -1.4 |
| H39 | 0.4 | -2.0 | -2.5 | -1.4 |
| H40 | 0.2 | -2.2 | -3.2 | -1.8 |
| H41 | 0.2 | -2.2 | -3.2 | -1.8 |
| H42 | -0.4 | -0.7 | 0.9 | -0.1 |
| H43 | -0.4 | -0.7 | 0.9 | -0.1 |
| H44 | -0.3 | -0.5 | 0.9 | 0.1 |

| Center | $A_{min}$ | $A_{mid}$ | $A_{max}$ | $A_{iso}$ |
|---|---|---|---|---|
| H45 | -0.3 | -0.5 | 0.9 | 0.1 |

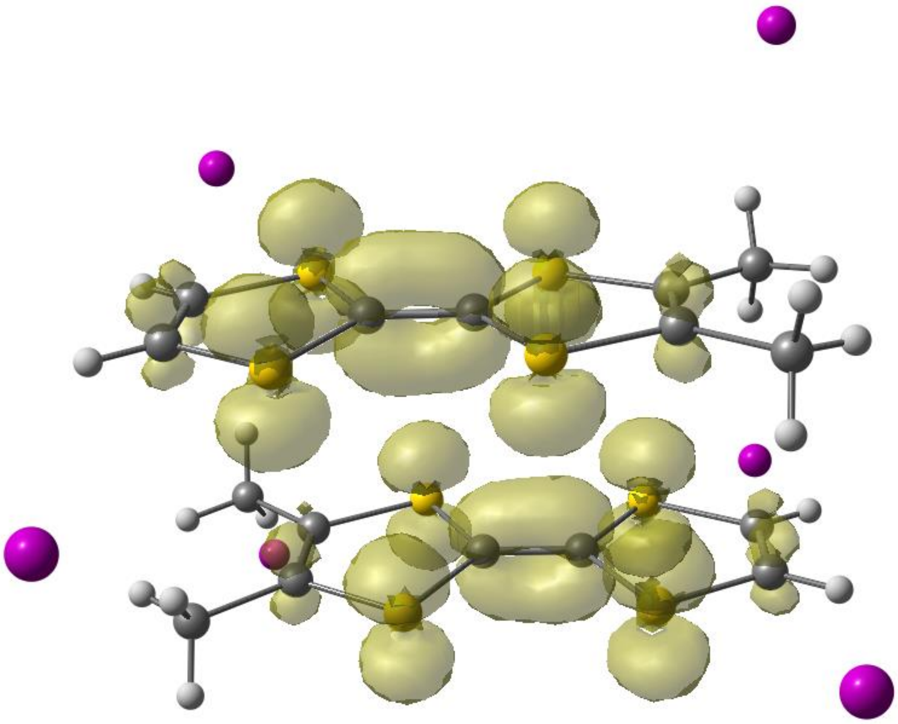

**Spin density plot**

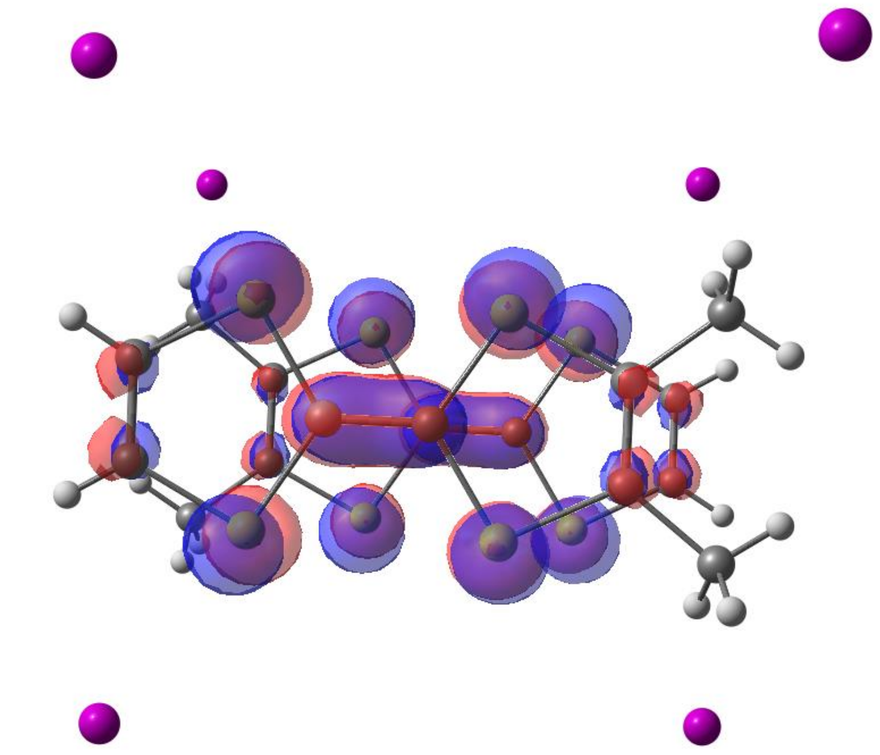

**Singly Occupied Molecular Orbital**

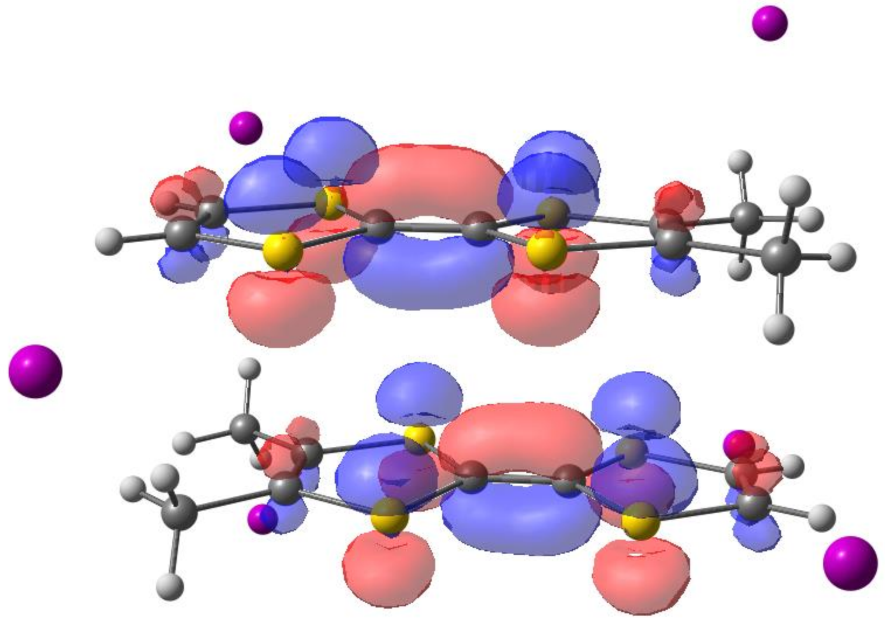

**Singly Occupied Molecular Orbital**

**NMR properties**

# Larmor frequencies

| Isotopes | Natural abundance (%) | Larmor frequency (MHz) $H_0 = 3454$ G | Larmor frequency relative to $^1H$ (%) | Nuclear spin I |
|---|---|---|---|---|
| $^{1}$H | 99.9885 | 14.7 | 100 | 1/2 |
| $^{13}$C | 1.07 | 3.7 | 25.1504 | 1/2 |
| $^{14}$N | 99.636 | 1.06 | 7.2285 | 1 |
| $^{15}$N | 0.364 | 1.49 | 10.1398 | 1/2 |
| $^{29}$Si | 4.685 | 2.92 | 19.8826 | 1/2 |
| $^{33}$S | 0.75 | 1.13 | 7.6842 | 3/2 |
| $^{35}$Cl | 75.76 | 1.44 | 9.8093 | 3/2 |
| $^{37}$Cl | 24.24 | 1.20 | 8.1652 | 3/2 |
| $^{79}$Br | 50.69 | 3.70 | 25.1404 | 3/2 |
| $^{81}$Br | 49.31 | 3.98 | 27.0997 | 3/2 |
| $^{127}$I | 100 | 2.96 | 20.1462 | 5/2 |
| $^{129}$I | Unknown | 1.97 | 13.4067 | 7/2 |

Source : NMR Frequency Tables Bruker

**Crystallographic details**

| Anion (X) | X = I | X = Br | X = Cl |
|---|---|---|---|
| Formula | $C_{16}H_{16}I_1S_8$ | $C_{16}H_{16}Br_1S_8$ | $C_{16}H_{16}Cl_1S_8$ |
| Formula weight | 591.67 | 544.68 | 500.22 |
| Crystal system | Tetragonal | Tetragonal | Tetragonal |
| Space group | I42d | I42d | I42d |
| a/Å | 17.4031(2) | 17.0920(3) | 16.9376(6) |
| b/Å | 17.4031(2) | 17.0920(3) | 16.9376(6) |
| c/Å | 7.0978(1) | 7.0582(2) | 7.0400(3) |
| V/Å$^3$ | 2149.70(5) | 2061.96(8) | 2019.65(13) |
| T/K | 293(2) | 293(2) | 293(2) |
| Z | 4 | 4 | 4 |
| $\mu/mm^{-1}$ | 2.266 | 2.803 | 1.016 |
| Absorption corrections | multi-scan | multi-scan | multi-scan |
| $T_{min}$, $T_{max}$ | 0.3534, 0.8920 | 0.6393, 0.8301 | 0.8069, 1.1853 |
| Total reflections | 14532 | 17533 | 14655 |
| Unique reflections ($R_{int}$) | 1226 (0.0852) | 1191 (0.069) | 1161 (0.1299) |
| Unique reflections ( I > 2σ(I)) | 1197 | 1123 | 1010 |
| $R_1$, w$R_2$ $(I > 2\sigma(I))^a$ | 0.0229, 0.0575 | 0.024, 0.0578 | 0.0405, 0.0902 |
| $R_1$, w$R_2$ (all data))$^a$ | 0.0235, 0.0584 | 0.0271, 0.0596 | 0.0495, 0.0972 |
| Flack parameter | 0.00(3) | 0.378(12) | 0.3(2) |
| GOF | 1.087 | 0.953 | 0.914 |
| Residual density/e Å$^{-3}$ | +0.33, -0.66 | +0.25, -0.31 | +0.49, -0.37 |
